# Supplementary material for: Exchange bias effect in martensitic epitaxial Ni-Mn-Sn thin films applied to pin CoFeB/MgO/CoFeB magnetic tunnel junctions
Source: arXiv:1503.00440 source file (2015-05-07)
Supplement: Supplementary file 1 [file Supplementary_Material.pdf]

<u>Supplementary Material</u> to **'Exchange bias effect in martensitic epitaxial Ni-Mn-Sn thin films applied to pin CoFeB/MgO/CoFeB magnetic tunnel junctions'**

Niclas Teichert[1], Alexander Boehnke[1], Anna Behler[2], Bruno Weise[2], Anja Waske[2], and Andreas Hütten

[1]*Department of Physics, Center for Spinelectronic Materials and Devices, Bielefeld University, 33615 Bielefeld,*
[2]*IFW Dresden, Institute for Complex Materials, P.O. Box 270116, 01171 Dresden, Germany*

## 1. Structural properties of the Ni-Mn-Sn layer.

The crystal structure of the $Ni_{52}Mn_{34}Sn_{14}$ layer on single crystalline MgO(001) substrate (film B in the main article) was investigated using X-ray diffraction with Cu $K_\alpha$ radiation. A θ-2θ scan (cf. S 1(a)) reveals film growth in [001] direction because only the (002) and (004) reflection of the austenite phase of Ni-Mn-Sn are visible. The austenite lattice constant is $a_0 = 6.0$ Å. S 1(b) shows a 360° ϕ-scan of the (022) reflection (ψ=45°, 2θ=42.7°) using a 4-circle goniometer where ϕ=0 is the MgO[100] direction. It shows the 4-fold symmetry and reveals epitaxial growth with the relation MgO(001)[110]||Ni-Mn-Sn(001)[100]. S 1(c) shows the Ni-Mn-Sn(111) peak at ϕ=0° and ψ=54.74° which demonstrates that the film crystallizes in $L2_1$ structure. Structural investigation of the martensite phase of epitaxial Ni-Mn-Sn films with very similar composition is found in Ref. [1].

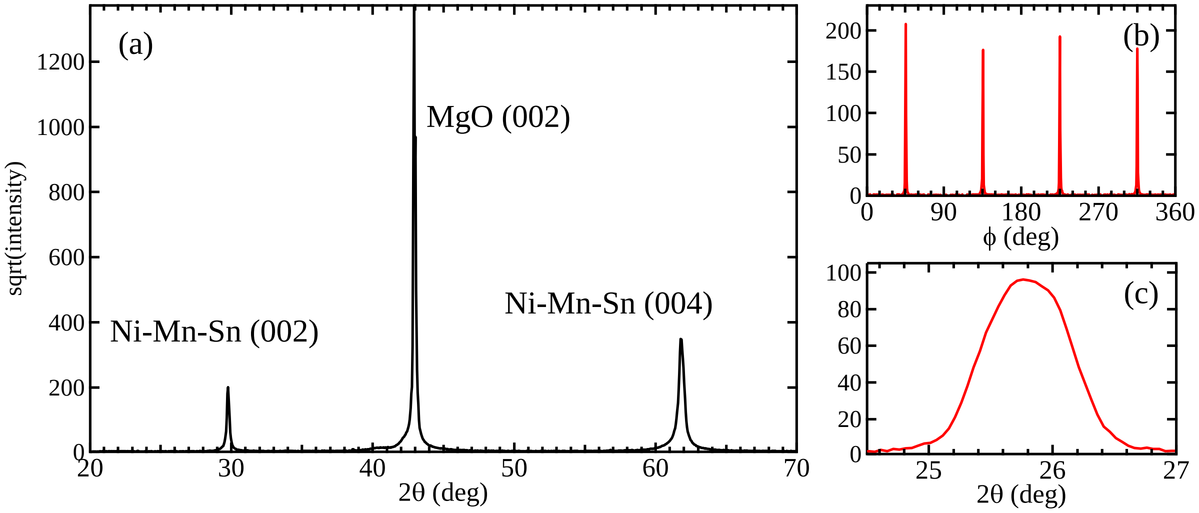


S 1 XRD patterns (Cu $K_\alpha$ radiation) of MgO(substrate)/$Ni_{52}Mn_{34}Sn_{14}$(220nm) at room temperature.(a) In the gonio-scan the (004) and (002) peaks of the austenite phase are observed together with the MgO(002) peak. (b) 360° ϕ-scan of the Ni-Mn-Sn(022) peak at ψ=45° and 2θ=42.7° reveals epitaxial growth. (c) The 2θ-scan of the Ni-Mn-Sn(111) peak at ϕ=0° and ψ=54.74° shows that the film crystallizes in $L2_1$ structure.

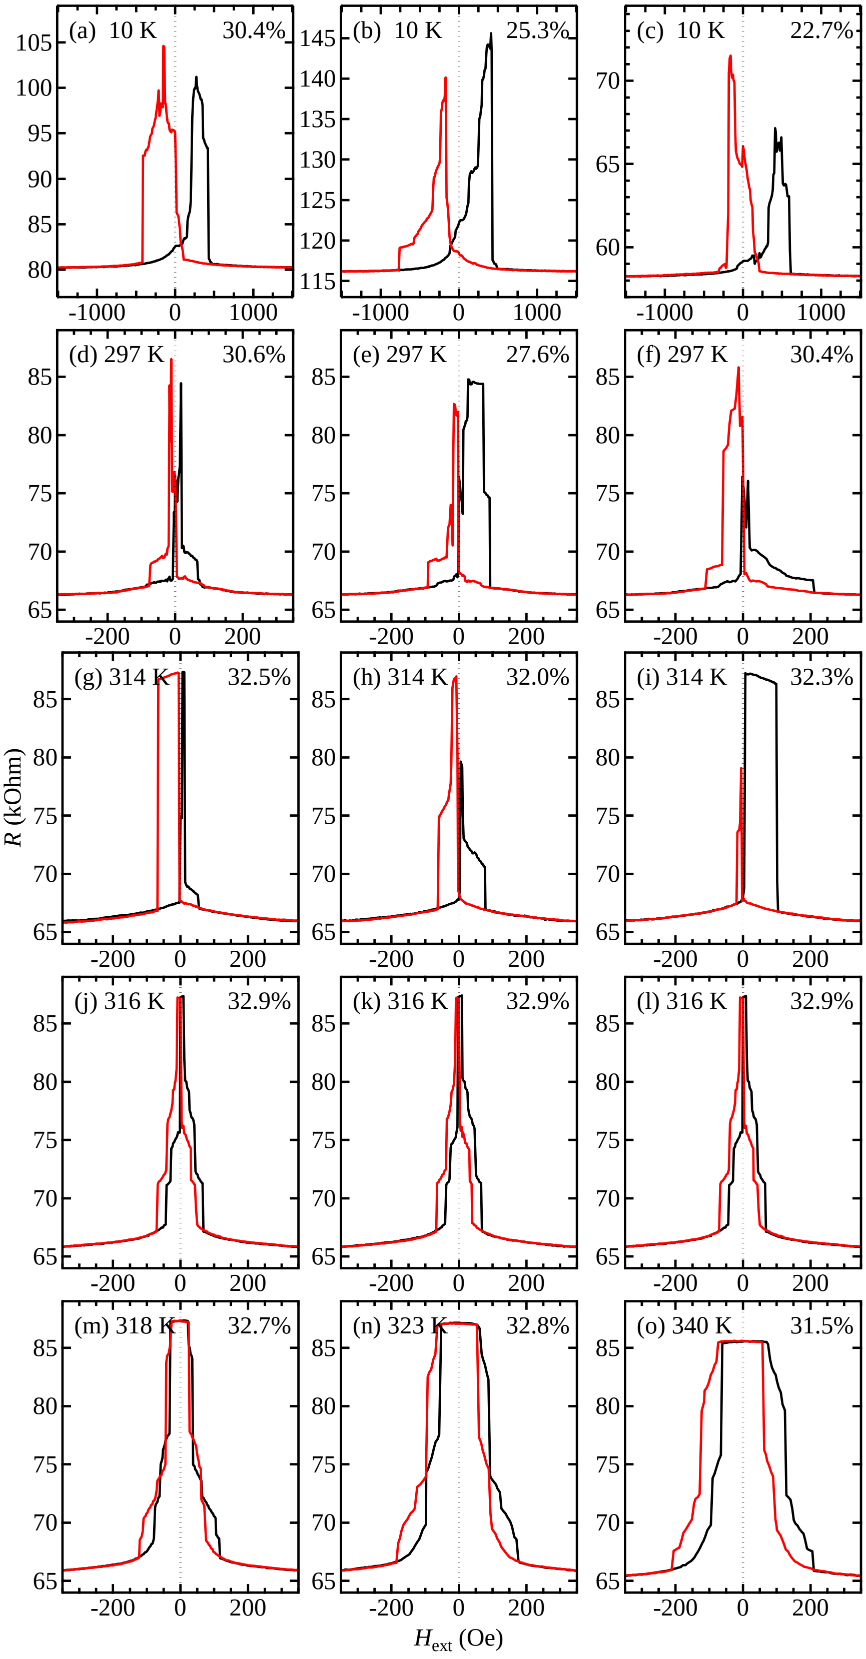


S 2 Tunnel magnetoresistance at different temperatures. (a)-(c) TMR curves of different MTJs at 10 K. Successively measured TMR curves of the same MTJ at (d)-(f) 297 K, (g)-(i) 314 K, and (j)-(l) 316 K. (m), (n), (o) TMR at 318 K, 323 K, and 340 K, respectively. The TMR amplitude is given in the upper right corner. Black and red lines denote increasing and decreasing field, respectively. At low temperature the shape of the curves is non-reproducible but the exchange bias effect is clearly visible. When the Ni-Mn-Sn layer is austenitic and ferromagnetic the TMR curves are highly asymmetric and non-reproducible (d)-(i). Above the curie temperature of the austenite the TMR curves are symmetric and reproducible, and show antiparallel coupling at zero external field.

## 2. Temperature dependence of the tunnel magnetoresistance

S 2 shows tunnel magnetoresistance (TMR) curves measured at different temperatures where at selected temperatures three sequentially measured loops are shown to demonstrate the non-reproducibility of the shape of the TMR curves. Up to 314 K all TMR curves are asymmetric and non-reproducible because the magnetic switching is dominated by Barkhausen jumps of the underlying Ni-Mn-Sn layer in which the domain walls move independently from the size and position of the magnetic tunnel junctions (MTJs). Also, in the martensite state (below $T_M$=256 K) the TMR curves always show spikes of maximum TMR instead of plateaus and non-reproducible TMR amplitudes (cf. also Fig. 3(a)-(c) in the main article). This clearly indicates that there is no fully antiparallel state of the magnetic electrodes present. This can be explained by the rather complex domain structure in the martensite phase. The domain size and orientation of magnetic easy axis is coupled to the size and orientation of martensitic variants in the film.[2] Based on the AFM micrograph in S3 of a structurally very similar 200nm thick epitaxial $Ni_{50}Co_1Mn_{36.5}Sn_{12.5}$ film which is martensitic (10M) at room temperature we expect a domain width of about 50 nm. Because adjacent variants have different orientations of magnetic easy axis it is likely that a fully antiferromagnetic state of the MTJ cannot be achieved. Despite this random influence the exchange bias effect at low temperatures is clearly observed (S 2(a)-(c)).

In the austenite phase below the Curie temperature of Ni-Mn-Sn ($T_c$ = 316 K) antiparallel states are observed but not reproducibly (S 2(d)-(i)). Antiparallel states are observed at low fields but not at zero field. The increased Barkhausen noise is probably attributed to an increased domain width in the austenite compared to the martensite.

The shape of the curves changes drastically above $T_c$ (S 2(j)-(o)): The TMR is symmetric and reproducible and at zero field the electrodes are aligned antiparallel. The plateau around zero field widens with increasing temperature. As described in the main article, this is caused by stray field coupling between the CoFeB layers when the Ni-Mn-Sn magnetization vanishes (compare also S 4).

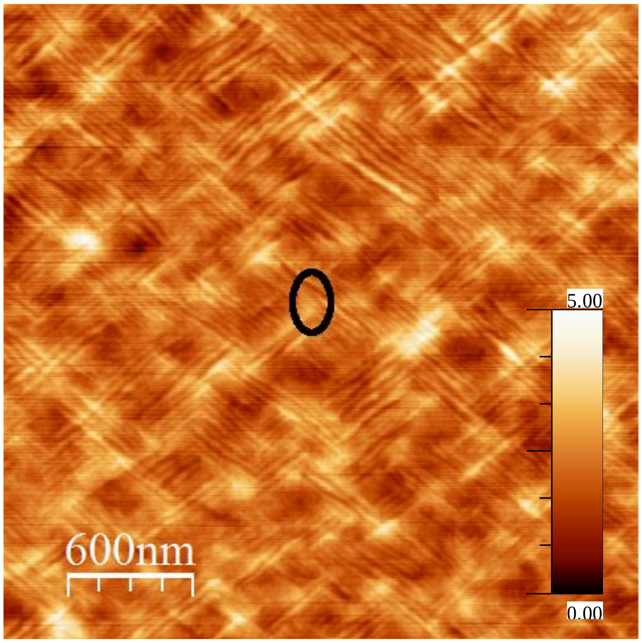


S 3 AFM micrograph of 200 nm thick epitaxial Ni-Co-Mn-Sn film at room temperature. The margins are parallel to the MgO[100] direction. The size of an MTJ is shown for scale as a black ellipse. The image shows traces of martensitic variants with a periodicity of approximately 50 nm. Therefore, the MTJ partly covers several martensitic variants.

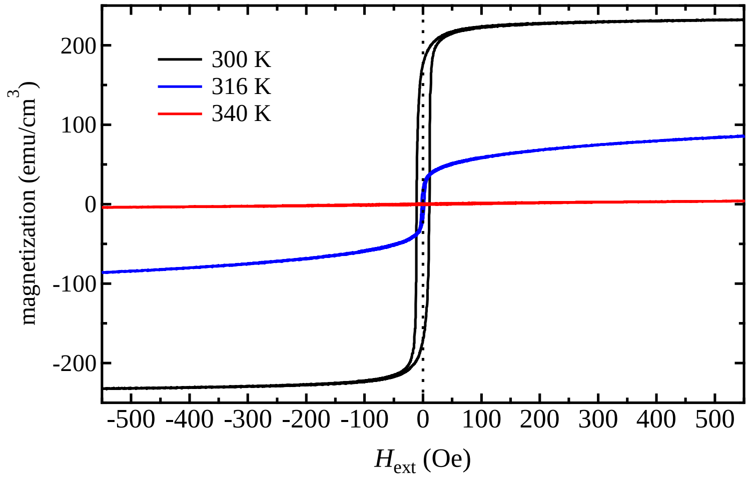


S 4 $M(T)$ measurements of 196 nm thick Ni-Mn-Sn film (sample B in the main article) around $T_C$=316 K.

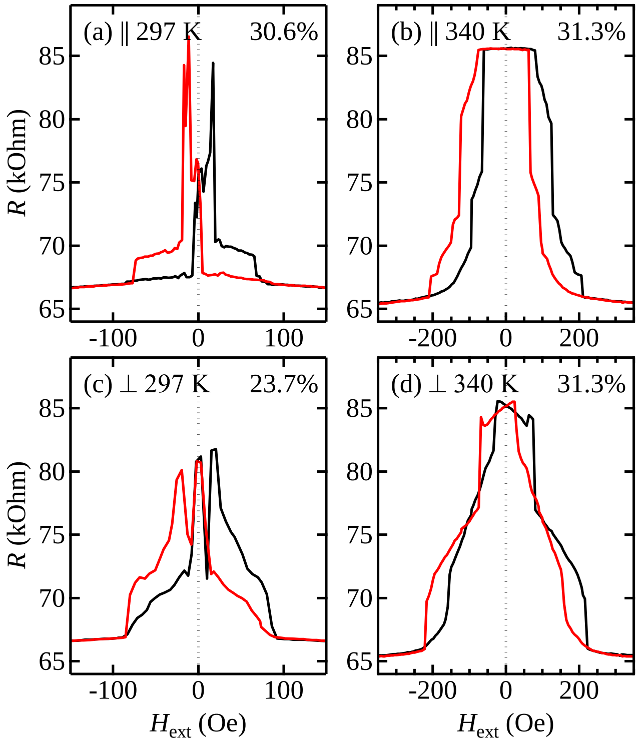


S 5 TMR curves with external field applied along the major axis (a)-(b) and minor axis (c)-(d) of the ellipsoidal MTJs. Black and red lines denote increasing and decreasing external field, respectively. The TMR amplitude is given in the upper right corner.

# 3. Shape anisotropy of ellipsoidal MTJs

Due to the ellipsoidal shape and the accompanying shape anisotropy of the MTJs we observe different TMR curves depending on the direction of the external magnetic field. In S 5 the TMR under different directions of the external field are compared for two different temperatures. In S 5(a) and (b) the external field is applied parallel to the major axis and in S 5(c) and (d) parallel to the minor axis of the ellipsoids.

For both temperatures an external field applied along the minor (hard) axis instead of the major (easy) axis leads to broader TMR curves and more gradual magnetic switching due to the shape anisotropy of the ellipsoidal MTJs. Furthermore, S 5(c) and (d) show two maxima for each field direction where the maximum near zero field corresponds to (partly) antiparallel configuration along the major axis and the other maximum corresponds to partly antiparallel configuration along the minor axis, presumably.

# References.

[1] N. Teichert, A. Auge, E. Yüzüak, I. Dincer, Y. Elerman, B. Krumme, H. Wende, O. Yildirim, K. Potzger, and A. Hütten, Acta Mater. **86**, 279 (2015).

[2] A. Diestel, A. Backen, V. Neu, L. Schultz, and S. Fähler, Scripta Mater. **67**, 423 (2012).
